# Supplementary material for: WhatELSE: Shaping Narrative Spaces at Configurable Level of Abstraction for AI-bridged Interactive Storytelling
Source: arXiv:2502.18641 source file (2025-02-25)
Supplement: Supplementary file 1 [file appendix.tex]

\section{Variants to Interactive Narrative}
\label{variants_to_graph}

% Using the following algorithm, we can transfer the variants to a list of event graphs. Thus, the generation of game plots becomes a traditional planning problem with LLM generation of character behavior. 

In this section, we describe a tentative approach to transfer the variant plots generated by \textsc{WhatELSE} to an event diagram for interactive narrative creation.

\subsection{Event Evaluation Function \( F \)}

We first define a function \( F(E_1, E_2) \) that returns \textbf{True} if and only if events \( E_1 \) and \( E_2 \) are the same, otherwise it returns \textbf{False}:

\[
F(E_1, E_2) =
\begin{cases}
\text{True}, & \text{if } E_1 = E_2 \\
\text{False}, & \text{otherwise}
\end{cases}
\]

This function can be implemented by traditional event extraction technologies or more conveniently using LLM prompting judgments.

\subsection{An algorithm to generate plot graphs}

\textbf{Input:}
\begin{itemize}
    \item \( \mathcal{P} = \{P_1, P_2, \dots, P_N\} \): A set of \( N \) variants, where each \( P_i \) is a linked list of event nodes.
\end{itemize}

\textbf{Output:}
\begin{itemize}
    \item \( \mathcal{G} = \{G_1, G_2, \dots, G_K\} \): A set of \( K \) graphs, where each graph is a set of event nodes.
\end{itemize}

\textbf{Symbols:}
\begin{itemize}
    \item \( \text{event\_to\_graph} \): A dictionary that maps each event node \( E \) to a graph index.
    \item \( \mathcal{G} \): A list of graphs, where each graph \( G \) is a set of event nodes.
    \item \( \text{graph\_indices} \): A set that stores the indices of graphs related to the current path.
    \item \( F(E_1, E_2) \): A function that returns \textbf{True} if two event nodes \( E_1 \) and \( E_2 \) are the same, otherwise returns \textbf{False}.
\end{itemize}

\textbf{Algorithm:}

\begin{algorithm}
\caption{Merge Narrative Paths to Narrative Graphs}
\begin{algorithmic}[1]
\State \textbf{Initialize} \( \text{Event to graph dictionary: } \mathcal{D} \leftarrow \emptyset, \text{Merged Graphs}: \mathcal{G} \leftarrow \emptyset \)

\For{each \( P_i \) in \( \mathcal{P} \)}
    \State \textbf{Initialize} \( \text{graph\_indices: } \mathcal{I} \leftarrow \emptyset \)

    \For{each event \( E_j \) in \( P_i \)}
        \For{each \( E_k \) in \(\mathcal{D} \)}
            \If{\( F(E_j, E_k) \) is \textbf{True}}
                \State Add \( \mathcal{D}[E_k] \) to \( \mathcal{I} \)
            \EndIf
        \EndFor
    \EndFor

    \If{\( |\mathcal{I}| > 1 \)}
        \State \textbf{Initialize} \( \mathcal{G'} \leftarrow \emptyset \)
        \For{each \( g \) in \( \mathcal{I} \)}
            \State Add all nodes from \( \mathcal{G}[g] \) to \( \mathcal{G'} \)
            \State Remove \( \mathcal{G}[g] \)
        \EndFor

        \State Add all nodes from \( P_i \) to \( \mathcal{G'} \)
        \State Append \( \mathcal{G'} \) to \( \mathcal{G} \)
        \For{each event \( E_j \) in \( \mathcal{G'} \)}
            \State \( \mathcal{D}[E_j] \gets \) index of \( \mathcal{G'} \) in \( \mathcal{G} \)
        \EndFor

    \ElsIf{\( |\mathcal{I}| = 1 \)}
        \State Let \( g \) be the single graph index in \( \mathcal{I} \)
        \State Add all nodes from \( P_i \) to \( \mathcal{G}[g] \)
        \For{each event \( E_j \) in \( P_i \)}
            \State \( \mathcal{D}[E_j] \gets g \)
        \EndFor

    \Else
        \State \textbf{Initialize} \( \text{new\_graph} \leftarrow \{E_j : E_j \in P_i\} \)
        \State Append \( \text{new\_graph} \) to \( \mathcal{G} \)
        \For{each event \( E_j \) in \( P_i \)}
            \State \( \mathcal{D}[E_j] \gets \) index of \( \text{new\_graph} \) in \( \mathcal{G} \)
        \EndFor
    \EndIf
    
\EndFor

\State \textbf{Return} \( \mathcal{G} \)
\end{algorithmic}
\end{algorithm}
